# Supplementary material for: A Local-Global Approach to Semantic Segmentation in Aerial Images
Source: arXiv:1607.05620 source file (2016-07-19)
Supplement: Supplementary file 2 [file build.system.makefiles.tex]

\chapter{Project Build System Makefiles}

% All this appendix uses make syntax
\lstset{language=make}

\section{Makefile.test}

\lstset{caption=Testing Targets Makefile (Makefile.test), label=lst:makefile-test}
\lstinputlisting{src/code/build/Makefile.test}
